# Supplementary material for: SurfaceNet: An End-to-end 3D Neural Network for Multiview Stereopsis
Source: arXiv:1708.01749 source file (2017-08-05)
Supplement: Supplementary file 1 [file appendix.tex]

\begin{appendices}
\newpage

%=========================================================================
\section{appendix} \label{appendix}

how the choose the train/val/test set in DTU dataset

more figures 

\end{appendices}
